# Supplementary material for: Platform-Driven Collaboration Patterns: Structural Evolution Over Time and Scale
Source: arXiv:2402.12686 source file (2024-02-23)
Supplement: Supplementary file 1 [file Appendix.pdf]

**Appendix Document**

# Platform-Driven Collaboration Patterns: Structural Evolution Over Time and Scale

Negin Maddah, Babak Heydari
Department of Mechanical and Industrial Engineering, Northeastern University,
Network Science Institute, Boston, MA 02115, United States

## 1- General Information: Sample Data

Here is a list of all the sample articles within each category used in the analysis:

*Table 1. Sample Articles of Wikipedia per Category*

| | Category | Sample topics |
|---|---|---|
| 1 | Political Figures and Events | 'Pete Buttigieg',<br>'Sanna Marin',<br>'Emmanuel Macron',<br>'Abiy Ahmed',<br>'Ron DeSantis',<br>'Alexandria Ocasio-Cortez',<br>'Jair Bolsonaro',<br>'Volodymyr Zelenskyy',<br>'Brexit negotiations',<br>'Impeachment inquiry against Donald Trump',<br>'2020 Democratic Party presidential primaries',<br>'Jacinda Ardern', |
| 2 | International Conflicts | 'Syrian Civil War',<br>'2019–2020 Hong Kong protests',<br>'Assassination of Qasem Soleimani',<br>'Annexation of Crimea by the Russian Federation',<br>'Ferguson unrest',<br>'Rohingya genocide',<br>'Russo-Ukrainian War',<br>'Nagorno-Karabakh conflict',<br>'Yemeni civil war (2014–present)',<br>'Battle of Mosul (2016–2017)',<br>'2019 India–Pakistan border skirmishes',<br>'Operation Olive Branch',<br>'Insurgency in Cabo Delgado', |
| 3 | Natural and Man-Made Disasters | 'COVID-19',<br>'Zika virus',<br>'2010 Haiti earthquake',<br>'April 2015 Nepal earthquake',<br>'2018 California wildfires',<br>'2019–20 Australian bushfire season',<br>'2019 Amazon rainforest wildfires',<br>'Cyclone Idai',<br>'2020–2022 Taal Volcano eruptions',<br>'Hurricane Harvey',<br>'2018 Sulawesi earthquake and tsunami',<br>'Hurricane Dorian',<br>'2020 Beirut explosion',<br>'2021 Suez Canal obstruction', |

| | | |
|---|---|---|
| 4 | Technology and Business | 'Tesla Model 3',<br>'Non-fungible token',<br>'5G',<br>'E-commerce in India',<br>'Cryptocurrency',<br>'TikTok',<br>'Neuralink',<br>'Quantum cryptography',<br>'Zoom Video Communications',<br>'Tesla Cybertruck',<br>'COVID-19 apps',<br>'Starlink', |
| 5 | Entertainment | 'Moonlight (2016 film)',<br>'Parasite (2019 film)',<br>'Billie Eilish',<br>'Kylian Mbappé',<br>'Erling Haaland',<br>'2022 FIFA World Cup',<br>'BTS',<br>'Squid Game',<br>'Black Panther (film)',<br>'Chernobyl (miniseries)',<br>'Joker (2019 film)',<br>'Megan Thee Stallion',<br>'Old Town Road' |

## 2- **Distribution of the Temporal (ATI) and Content Weights**

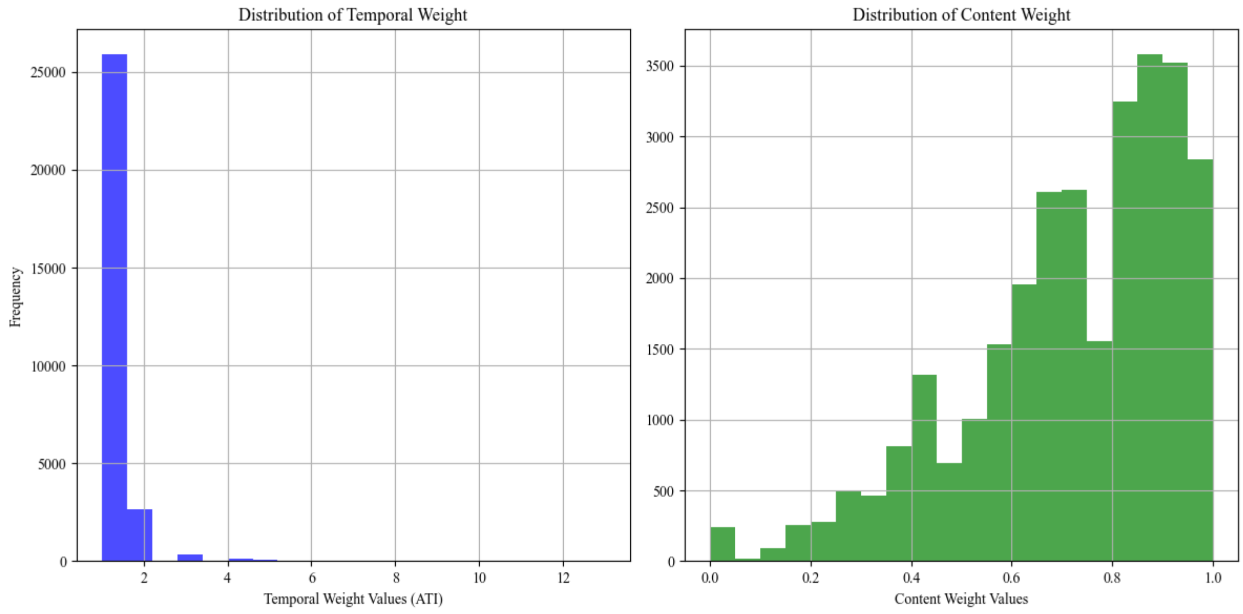


*Figure 1. Distributions of Temporal and Content Weights of Wikipedia Collaborators*

The visualization of temporal weights and content weights among all 29,149 pairs of editors, who collaborate on Wikipedia articles, in Figure 1, reveals insightful trends in collaborative behaviors and content alignment. The distribution of temporal weights predominantly showcases a concentration of values at 1, with a smaller yet notable presence of values at 2, and scarcely any values exceeding 4 to 12. This distribution pattern underscores a

predominant trend of editors engaging in two consecutive activities within the defined 48-hour threshold, as captured by the Alternating Timed Interaction (ATI) metric (explained in the Methodology section).

Further refinement in understanding these collaborative dynamics comes from adjusting these temporal weights with content weights, which are normalized over the total number of sub-sections for each article. The range of these content weights is between 0 and 1, serving as a filter to emphasize connections that are not only temporally proximate but also contextually relevant—those that signify meaningful content similarity. The distribution of content weights exhibits a right-skewed pattern, indicating that while most editor pairs have higher content similarity, there is a long tail of pairs with small similarity.

The dual-layered analysis of collaborators' connections reflects a landscape where immediate interactions are common but are filtered through the lens of content relevance, ensuring that the collaborations that persist and are highlighted through these weights are both timely and contextually coherent.

## 3- Sample Data Summary Before Filtering the Pre-Active Time-Windows

Figure 2 is a visual representation of our domain selection, showcasing the distribution of the sample articles across each category and highlighting the creation dates of these articles before filtering out the pre-active time windows. Similarly, Table 2 presents other details regarding the dataset used for the network analysis before filtering.

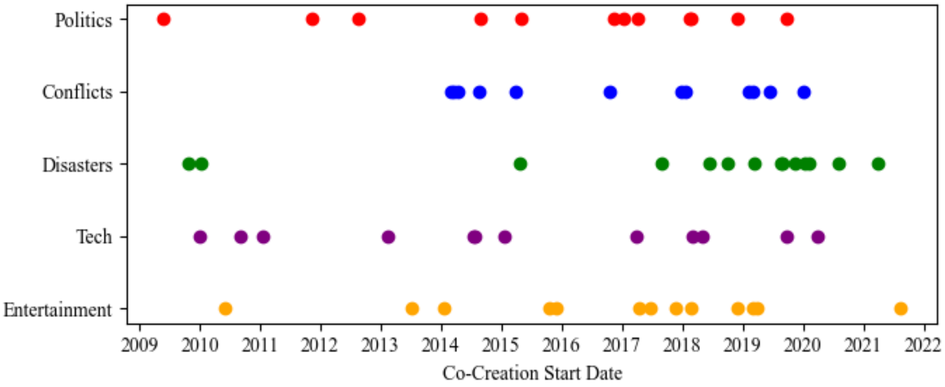


*Figure 2. The temporal distribution and the number of sample articles selected for each category before filtering the pre-active time*

*Table 2. Summary of Constructed Networks by category (for all the networks before filtering the pre-active time)*

| **Category** | **#Topics** | **#Networks** | **Min Start Date** | **Max End Date** | **Min #Nodes** | **Max #Nodes** |
|---|---|---|---|---|---|---|
| Politics | 12 | 168 | 2009-05-28 00:18:34+00:00 | 2023-11-30 22:57:44+00:00 | 2 | 29 |
| Conflicts | 12 | 155 | 2014-03-01 23:01:38+00:00 | 2023-12-23 17:07:20+00:00 | 2 | 27 |
| Disasters | 14 | 145 | 2009-10-25 21:51:24+00:00 | 2023-12-10 21:02:50+00:00 | 2 | 27 |
| Tech | 12 | 192 | 2010-01-03 08:46:49+00:00 | 2023-11-02 21:03:38+00:00 | 2 | 31 |
| Entertainment | 13 | 179 | 2010-06-03 00:19:30+00:00 | 2023-12-18 13:54:27+00:00 | 2 | 36 |

## 4- Pre-Active Time-Window filtering

Upon examining the patterns of editorial activity across our dataset of Wikipedia articles, we determined a threshold for significant collaborative engagement. Our analysis revealed that removing the early, less active stage—referred to as the pre-active era—until the number of active editors reaches 15% of an article's peak engagement level, accurately reflects periods of meaningful collaboration for the majority of our sample articles. This threshold was chosen based on its relevance and applicability across various topics, ensuring that our focus remains on time windows characterized by substantial editorial activity. This allows for a meaningful understanding of the collaborative dynamics, emphasizing the phases of interaction that truly contribute to the article's development. The formative stages of an article, while foundational, often do not represent the full extent of collaborative effort it garners over time.

Here are two examples in Figures 3 and 4 that show the trend of the number of collaborators and how the pre-active phase has been filtered out of the rest of the analysis for “Ron DeSantis” in the politics category and “Kylian Mbape” in the entertainment domain. The activation of collaborations on Wikipedia pages is usually a reflection of the public interest or engagement of people in real-life events or circumstances. It should be mentioned that “nn_GCC” is the number of nodes for the Giant Connected Component of the network per each 6-month timeframe.

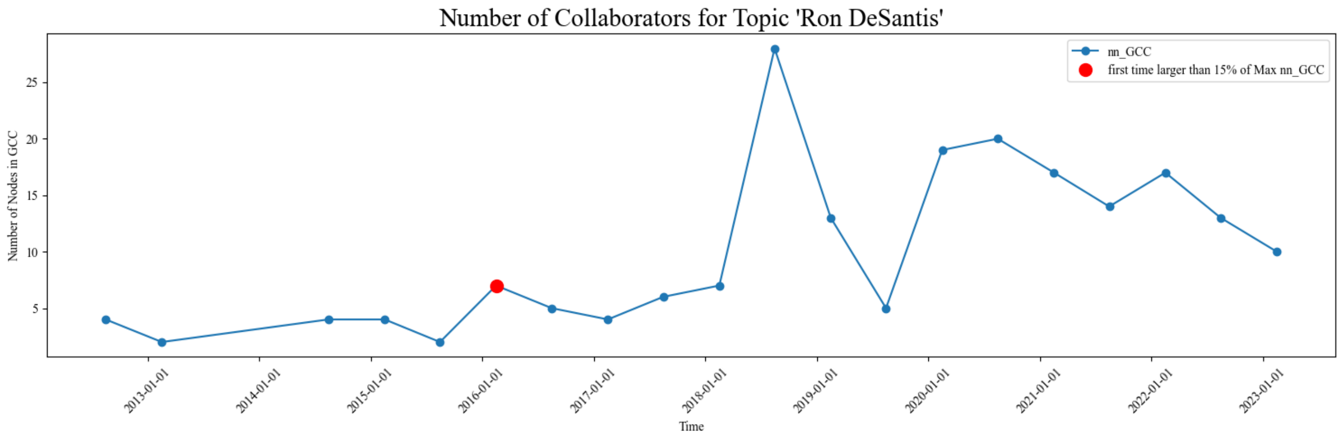


*Figure 3. The trend of collaborators count over time for the article: Ron DeSantis*

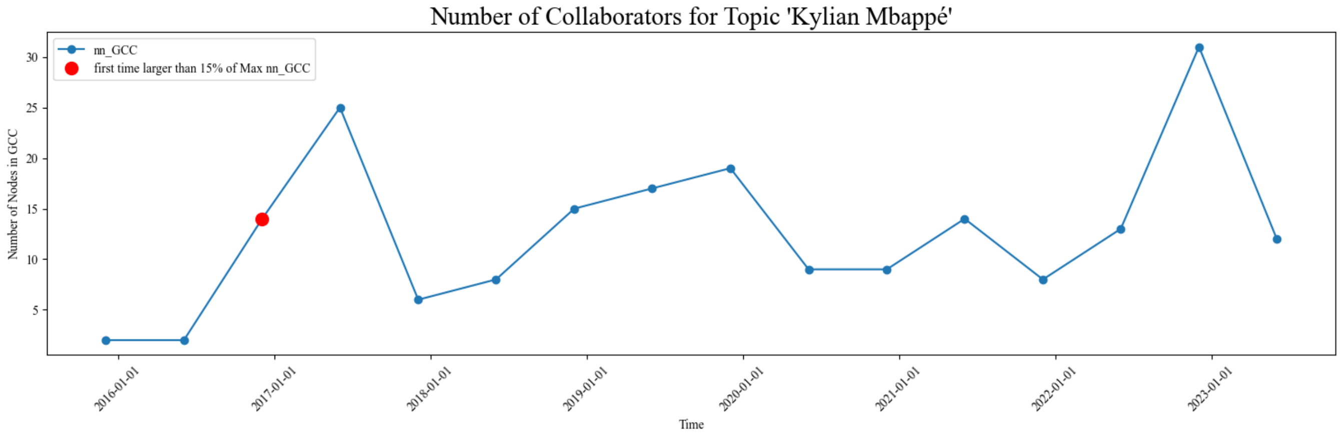


*Figure 4. The trend of collaborators count over time for the article: Kylian Mbappe*

These instances underscore the rationale behind selecting the 15% threshold for pre-active time-window filtering, demonstrating its effectiveness in isolating the active phases of collaboration across our dataset. By applying this approach, we ensure that the analysis is grounded in periods of editorial activity that are both significant and representative of the articles' evolving narrative.

## 5- Network Characteristics Distribution

Figure 5 shows the distribution characteristics of several network metrics across the studied categories. Notably, the average degree distribution is markedly left-skewed, featuring a long tail that indicates a predominance of networks with connectivity below 5, while only a minority exhibit an average degree above this threshold. Conversely, the clustering coefficient and average shortest path length display distributions that approximate normality across all categories, centering around mean values of 1.7 and 0.6, respectively. This suggests a relatively uniform pattern of local clustering and network reachability within these networks. Betweenness centrality presents a left-tailed distribution with a mean of 0.095, highlighting that most nodes have lower betweenness scores, indicating fewer nodes act as principal bridges within their respective networks. Similarly, the distributions for the number of nodes and the age of networks are left-tailed, with the data revealing an average of 11 collaborators per network and a typical network age of 42 months. These distributions underscore the variability in network dynamics and structure within the dataset. Detailed summary statistics supporting these observations are provided in Table 4, offering a comprehensive overview of the network properties examined.

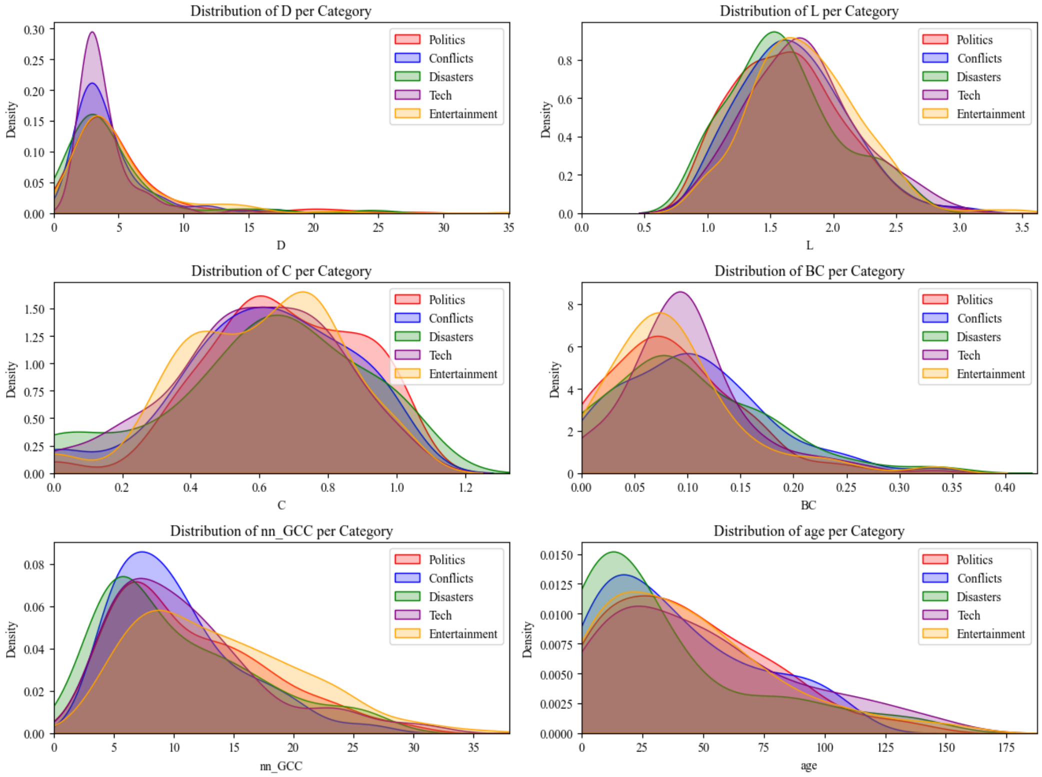


*Figure 5. The Distribution of Network Metrics*

*Table 3. Summary Statistics of the Characteristics of the Networks Constructed*

| | #Nodes | Age | D | L | C | BC | Edge Ratio |
|---|---|---|---|---|---|---|---|
| **count** | 651.000 | 651.000 | 651.000 | 651.000 | 651.000 | 651.000 | 651.000 |
| **mean** | 11.538 | 42.711 | 4.677 | 1.704 | 0.616 | 0.095 | 0.968 |
| **std** | 6.320 | 35.296 | 3.892 | 0.441 | 0.244 | 0.066 | 0.076 |
| **min** | 4.000 | 0.000 | 1.500 | 1.000 | 0.000 | 0.000 | 0.600 |
| **25%** | 6.000 | 12.000 | 2.686 | 1.393 | 0.462 | 0.050 | 1.000 |

| | #Nodes | Age | D | L | C | BC | Edge Ratio |
|---|---|---|---|---|---|---|---|
| **50%** | 10.000 | 37.000 | 3.385 | 1.667 | 0.628 | 0.087 | 1.000 |
| **75%** | 15.000 | 61.000 | 5.000 | 1.956 | 0.789 | 0.127 | 1.000 |
| **max** | 36.000 | 158.000 | 35.000 | 4.512 | 1.000 | 0.333 | 1.000 |

## 6- Team Structures Patterns Including the Scatter Data Points

Although the trends of the network structures over scale and time are presented in the main manuscript, here is another version of the same results including the networks' data points in Figure 6.

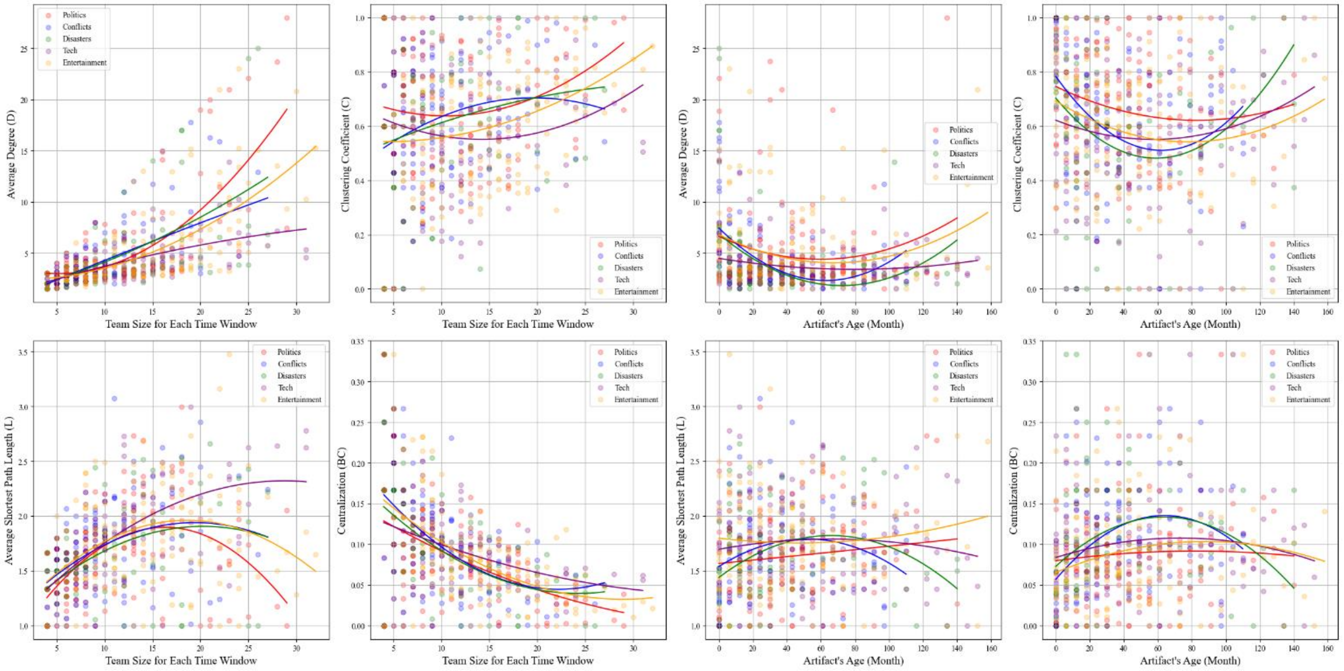


*Figure 6. Network Structure Patterns When the Teams Grow in Size per Artifacts Category: each collaboration team is defined per 6-month time windows from the onset of the meaningful interactions until the end of 2023. A 48-hour time threshold is set for measuring the ATI weights.*

## 7- Robustness Check for Lower Time Threshold

In assessing the impact of varying time thresholds on the calculation of temporal weights among editor pairs, we initially adopted a 48-hour criterion, as delineated in the Methodology and Results sections of our study. This criterion posits that an edge, with a weight of 1, is established between two editors following sequential interactions that occur within this 48-hour window. To further test the resilience of observed patterns, we subsequently adjusted this threshold to 24 hours. Illustrated in Table 5, this adjustment revealed that two specific relationships lost their statistical significance with age, underscoring the sensitivity of political topics to the reduced threshold (colored in red in Table 5). Despite these variances, the overarching findings of our research demonstrate considerable stability, even with the application of a more stringent 24-hour threshold for temporal interactions. This robustness reinforces the validity of the patterns and conclusions presented in our paper, affirming the consistency and reliability of our analysis as depicted in Figure 7.

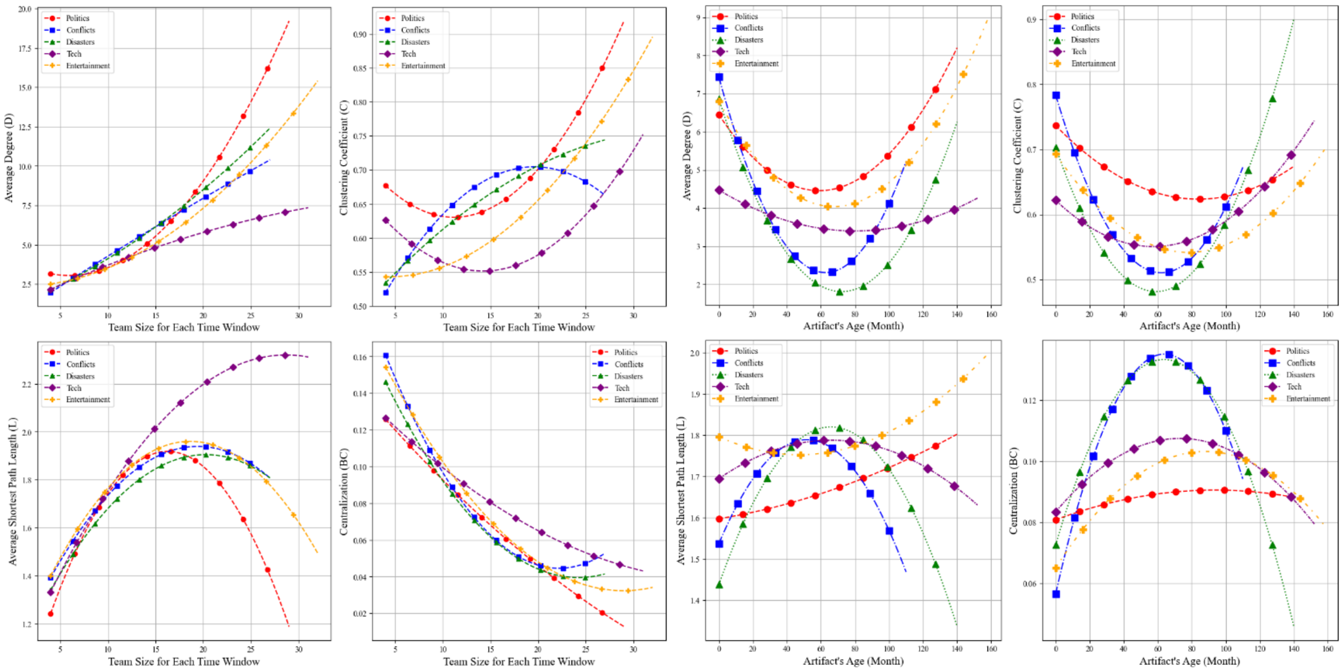


*Figure 7. Network Characteristics Trends over Scale (Size) and Time (Age) Excluding the Data Point of the Networks for 24-hour Time Threshold Measuring ATI weights.*

*Table 4. The Results of Regression Models of Structure Metrics vs Scale (size) of the teams and the time (age) of the Artifacts (for a 24-hour time threshold)*

| **Network Metric** | **Category** | **Scale** | | | | **Time** | | | |
|---|---|---|---|---|---|---|---|---|---|
| | | **Size** | $\boldsymbol{Size^2}$ | **Prob(F)** | **Adj $R^2$** | **Age** | $\boldsymbol{Age^2}$ | **Prob(F)** | **Adj $R^2$** |
| Average Degree (D) | Politics | 0.344 | ≪ 0.001 * | ≪ 0.001 * | 0.549 | 0.069 | 0.069 | 0.181 | 0.011 |
| | Conflicts | ≪ 0.001* | 0.768 | ≪ 0.001* | 0.480 | ≪ 0.001* | ≪ 0.001* | ≪ 0.001* | 0.280 |
| | Disasters | 0.016* | 0.430 | ≪ 0.001* | 0.483 | ≪ 0.001* | 0.003* | 0.001* | 0.124 |
| | Tech | ≪ 0.001* | 0.005* | ≪ 0.001* | 0.484 | 0.079 | 0.140 | 0.175 | 0.011 |
| | Entertainment | 0.044* | ≪ 0.001* | ≪ 0.001* | 0.555 | ≪ 0.001* | ≪ 0.001* | 0.001* | 0.071 |
| Clustering Coefficient (C) | Politics | 0.005* | 0.075 | ≪ 0.001* | 0.119 | 0.135 | 0.292 | 0.186 | 0.011 |
| | Conflicts | ≪ 0.001* | 0.001* | ≪ 0.001* | 0.163 | ≪ 0.001* | 0.002 | ≪ 0.001* | 0.111 |
| | Disasters | ≪ 0.001* | 0.002* | ≪ 0.001* | 0.187 | 0.005* | 0.004* | 0.014* | 0.075 |
| | Tech | ≪ 0.001* | 0.016* | ≪ 0.001* | 0.084 | 0.159 | 0.098 | 0.220 | 0.008 |
| | Entertainment | 0.806 | 0.345 | ≪ 0.001* | 0.102 | 0.005* | 0.018* | 0.013* | 0.040 |
| Average Shortest Path Length (L) | Politics | ≪ 0.001* | ≪ 0.001* | ≪ 0.001* | 0.379 | 0.843 | 0.847 | 0.513 | -0.005 |
| | Conflicts | ≪ 0.001* | ≪ 0.001* | ≪ 0.001* | 0.389 | 0.017* | 0.017* | 0.053 | 0.031 |

| Network Metric | Category | Scale | | | | Time | | | |
|---|---|---|---|---|---|---|---|---|---|
| | | Size | $Size^2$ | Prob(F) | Adj $R^2$ | Age | $Age^2$ | Prob(F) | Adj $R^2$ |
| | Disasters | ≪ 0.001* | ≪ 0.001* | ≪ 0.001* | 0.511 | 0.004* | 0.007* | 0.016* | 0.072 |
| | Tech | ≪ 0.001* | 0.003 | ≪ 0.001* | 0.598 | 0.221 | 0.208 | 0.450 | -0.003 |
| | Entertainment | ≪ 0.001* | ≪ 0.001* | ≪ 0.001* | 0.204 | 0.667 | 0.453 | 0.550 | -0.005 |
| Betweenness Centrality (BC) | Politics | 0.708 | 0.144 | ≪ 0.001* | 0.097 | 0.690 | 0.802 | 0.861 | -0.013 |
| | Conflicts | 0.303 | 0.069 | 0.011 | 0.045 | ≪ 0.001* | 0.002 | ≪ 0.001* | 0.115 |
| | Disasters | 0.018* | 0.008* | 0.023 | 0.039 | 0.007* | 0.009* | 0.026* | 0.061 |
| | Tech | 0.427 | 0.178 | 0.119 | 0.013 | 0.100 | 0.128 | 0.254 | 0.006 |
| | Entertainment | 0.010* | 0.464 | ≪ 0.001* | 0.239 | 0.022* | 0.085 | 0.033* | 0.029 |
